# Supplementary material for: A spline-based spatial impulse response simulator
Source: arXiv:2110.15945 source file (2021-10-29)
Supplement: Supplementary file 1 [file supmat-commands.tex]

\makeatletter
\newcommand*{\closecolumngrid}{\close@column@grid}
\makeatother

\makeatletter
\newcommand{\makesuptitle}{%
  \begin{flushleft}
    \textbf{\LARGE\@title: Supplementary material}
  \end{flushleft}
}
\makeatother

\def\enddocument{%
\listofchanges
\eject
\saveenddocument
}%

\newcommand{\supplements}{%
\phantomsection\label{finalpage}

\closecolumngrid
\clearpage

\setcounter{page}{1}%
\setcounter{section}{0}%
\setcounter{subsection}{0}%
\setcounter{subsubsection}{0}%
\setcounter{paragraph}{0}%
\setcounter{table}{0}%
\setcounter{figure}{0}%
\setcounter{equation}{0}%
\renewcommand{\theHsection}{Supplement.\thesection}%
\renewcommand{\theHtable}{Supplement.\thetable}%
\renewcommand{\theHfigure}{Supplement.\thefigure}%
\renewcommand{\theHequation}{Supplement.\theequation}%
\newcommand{\thesupplementprefix}{S}
\renewcommand{\thesection}{\thesupplementprefix-\Roman{section}}%
\renewcommand{\thetable}{\thesupplementprefix-\Roman{table}}%
\renewcommand{\thefigure}{\thesupplementprefix\arabic{figure}}%
\renewcommand{\theequation}{\thesupplementprefix\arabic{equation}}%

\makesuptitle
\onecolumngrid
}
